# Supplementary material for: Sonata: Query-Driven Network Telemetry
Source: arXiv:1705.01049 source file (2017-05-02)
Supplement: Supplementary file 1 [file appendix.tex]

\newpage
\appendix
\section{Algorithms}
\begin{algorithm}[t]
\begin{algorithmic}[1]
\Function{Gen-Hypothesis-Graphs}{${\boldsymbol Q}, {\boldsymbol T}$}
%\State $R = \Call{Get-Refinement-Levels}{Q}$
%\State $P = \Call{Get-Partitioning-Plans}{Q}$
%\State $L = \Call{Get-Iteration-Levels}{R}$
\State $V = \Call{Get-Vertices}{}$
\For {$m = 1$ \textbf{to} $M$}
\State $E_m = []$
\For{$(i,j) \in V.V$}
\State $ (r_i,p_i,l_i) = V_i, (r_j,p_j,l_j) = V_j$
\If{$l_{j} = l_{i}+1$ \& $r_{i} < r_{j}$}
  \State $b,n = \Call{Get-Cost}{Q, T_m, r_i,r_j, p_j}$
  \State $d$ = $1/|L|$
\State $\Call{Add-Edge}{E_m, V_i \rightarrow V_j, (b,n,d)}$
\EndIf
\EndFor
\State $G_m = (V,E_m)$
\EndFor
\State \Return $G$
\EndFunction
\end{algorithmic}
\caption{\label{alg:generate_graph} Generating Query Plan Graphs}
\end{algorithm}

\section{Monitoring Application Queries}
\label{sec:app-descr}
We present the code for the monitoring queries we discussed the paper
using \system's query interface. 
\subsection{Security Applications}
\smartparagraph{Detecting IP Address Spoofing}
Most of the reflection attacks are executed by sending the
requests messages with spoofed source IP address of the target~\cite{rossow}.
Fundamentally, address spoofing is possible as there is no check whether
information exchanged over control plane is realized in the data plane. 
Many solutions have been proposed to apply data
plane filters using control plane information. From streaming analytics
perspective, fusing the packet stream in the data plane with the routing
data is required to detect source address spoofing. Query~\ref{srcspoof-query} 
shows how a network operator can express such a query to detect presence
of source spoofing.

\noindent\begin{minipage}{\linewidth}
\begin{lstlisting}[language=Python,basicstyle=\footnotesize, 
caption= Query for detecting source IP address spoofing., 
captionpos=b, label=srcspoof-query, captionpos=b,
basicstyle=\footnotesize, 
numbers=left,xleftmargin=2em,frame=single,framexleftmargin=2.0em]
matched = pktStream(W)
  .filter(p => p.proto == 17)
  .map(p => (sMac, srcIP))
  .join(routing_data)
  .map(p => (srcIP, isMatch))
  .reduce(sum)
	
total = pktStream(W)
  .filter(p => p.proto == 17)
  .map(p => (srcIP,1))
  .reduce(sum)

spoofedstIPs = total
  .join(matched)
  .map(p => (srcIP, diff))
  .filter(diff > Th)
  .map(p => srcIP)
\end{lstlisting} 
\end{minipage}
\noindent

%\newpage

\smartparagraph{DNS Tunnel Detection}

\noindent\begin{minipage}{\linewidth}
\begin{lstlisting}[language=Python,basicstyle=\footnotesize, 
caption= Query for detecting DNS Tunneling~\cite{chimera}., 
captionpos=b, label=tunnel-query, captionpos=b,
basicstyle=\footnotesize, 
numbers=left,xleftmargin=2em,frame=single,framexleftmargin=2.0em]
observedDNS = pktStream(W1)
  .filter(p => p.sPort == 53)
  .map(p => (p.dstIP, p.dns.aIP))
  
totalConns = pktStream(W2)
  .map(p => (p.srcIP, p.dstIP))
  .distinct()
  
activeConns = observedDNS
	.join(totalConns)
  
dnsAIP = observedDNS
  .filter(p => (p not in activeConns))
  .map(p => (p.dstIP, 1))
  .reduce(sum)
  .filter(p => p.count > T)
  .map(p => p.dstIP)   
\end{lstlisting} 
\end{minipage}
\noindent

\smartparagraph{Spam Detection}
...

\noindent\begin{minipage}{\linewidth}
\begin{lstlisting}[language=Python,basicstyle=\footnotesize, 
caption= Query for Spam Detection~\cite{chimera}., 
captionpos=b, label=spam-query, captionpos=b,
basicstyle=\footnotesize, 
numbers=left,xleftmargin=2em,frame=single,framexleftmargin=2.0em]
newMTA = pktStream(W)
  .filter(isSMTP)
  .map(p => getMTA(p))
  .filter(isNew)
  .distinct()
  
spamMTA = pktStream(W)
  .filter(isSMTP)
  .map(p => (getMTA(p),p))
  .join(newMTA)
  .map((mta,p) => (recipient, mta))
  .distinct()
  .map(p => (p.mta,1))
  .reduce(sum)
  .filter(p => p.count > 50)
  .map(p => p.mta)
\end{lstlisting} 
\end{minipage}
\noindent

\smartparagraph{Sidejacking Detection}

\noindent\begin{minipage}{\linewidth}
\begin{lstlisting}[language=Python,basicstyle=\footnotesize, 
caption= Query for Sidejacking Detection~\cite{chimera}., 
captionpos=b, label=side-query, captionpos=b,
basicstyle=\footnotesize, 
numbers=left,xleftmargin=2em,frame=single,framexleftmargin=2.0em]
SessionIDs = pktStream(W)
  .filter(isHTTP)
  .map(p => (sessionID, userAgent))
  .distinct()
  .map(p => (p.sessionID, 1))
  .reduce(sum)
  .filter(p => p.count > 1)
  .map(p => p.sessionID)
\end{lstlisting} 
\end{minipage}
\noindent

\smartparagraph{SSH Brute Force Detection}

\noindent\begin{minipage}{\linewidth}
\begin{lstlisting}[language=Python,basicstyle=\footnotesize, 
caption= Query for detecting SSH brute forcing attacks~\cite{}., 
captionpos=b, label=ssh-query, captionpos=b,
basicstyle=\footnotesize, 
numbers=left,xleftmargin=2em,frame=single,framexleftmargin=2.0em]
victimIPs = pktStream(W)
  .filter(p => p.sPort = 22 or p.dPort = 22)
  .map(p => (p.dstIP, p.srcIP, p.size))
  .distinct()
  .map(p => ((p.dstIP, p.size),1))
  .reduce(sum)
  .filter(p => p.count > T)
  .map(p => p.dstIP)
\end{lstlisting} 
\end{minipage}
\noindent

\subsection{Performance Monitoring}
\smartparagraph{TCP Performance Monitoring}
...
\noindent\begin{minipage}{\linewidth}
\begin{lstlisting}[language=Python,basicstyle=\footnotesize, 
caption= Query for TCP Performance Monitoring., 
captionpos=b, label=perfmon-query, captionpos=b,
basicstyle=\footnotesize, 
numbers=left,xleftmargin=2em,frame=single,framexleftmargin=2.0em]
requests = pktStream(W)
  .filter(isApp && isRequest) 
  .map(p => (userGroup(p.srcIP), p.ts))
  .reduce(representative_stats)
						
responses = pktStream(W)
  .filter(isApp && isResponse) 
  .map(p => (userGroup(p.dstIP), p.ts)) 
  .reduce(representative_stats)
						
affected_users = requests
  .cogroup(responses) 
  .map(diff)
  .filter((UG, rtt) => rtt >T) 
  .map((UG, rtt) =>UG) 

local_bottlenecks = pktstream(W)
  .filter(isApp && isResponse)
  .join(affected_users)
  .map(p => ((inPort, outPort), (ql1, ql2,...)))
  .reduce(estimate pathMetric for each affected OD path)
  .filter(p => p.pathMetric > Tq)
  .map(p => (inPort, outPort))
\end{lstlisting} 
\end{minipage}
\noindent

{\tt isApp} leverages ideas described in NetAssay~\cite{} paper. We currently 
assume that it is possible to dynamically map an application to its 
header fields in real-time.
